# Supplementary material for: Learning Lane-Structured Conditioning Fields for Online HD Mapping
Source: arXiv:2610.25284 source file (2026-11-05)
Supplement: Supplementary file 2 [file preamble.tex]

%
% --- inline annotations
%
\newcommand{\red}[1]{{\color{red}#1}}
\newcommand{\todo}[1]{{\color{red}#1}}
\newcommand{\TODO}[1]{\textbf{\color{red}[TODO: #1]}}
% --- disable by uncommenting  
% \renewcommand{\TODO}[1]{}
% \renewcommand{\todo}[1]{#1}

%
% --- additional packages required by the paper content
%
\usepackage{multirow}
\usepackage{colortbl}
\usepackage[accsupp]{axessibility}  % Improves PDF readability for those with disabilities.

%
% --- collaborator annotation macros (legacy)
%
\newcommand{\tianyuan}[1]{{\color{red}{\scriptsize\textbf{Tianyuan: #1}}}}
\newcommand{\yicheng}[1]{{\color{blue}{\scriptsize\textbf{Yicheng: #1}}}}
\newcommand{\hang}[1]{{\color{red}{\scriptsize\textbf{Hang: #1}}}}
\newcommand{\yue}[1]{{\color{blue}{\scriptsize\textbf{Yue: #1}}}}
\newcommand{\yilun}[1]{{\color{red}{\scriptsize\textbf{Yilun: #1}}}}

\newcommand{\ADE}[1]{\textcolor{blue}{[\textbf{ADE}: #1]}}
\newcommand{\ANB}[1]{\textcolor{orange}{[\textbf{ANB}: #1]}}
\definecolor{TodoBlue}{RGB}{30,120,200}
\definecolor{TodoBlueBg}{RGB}{225,240,255}

\newcommand{\todotext}[1]{%
  {\color{TodoBlue}%
  \colorbox{TodoBlueBg}{\textbf{TODO:}}~#1}%
}
